# Supplementary material for: Online A-Optimal Design and Active Linear Regression
Source: arXiv:1906.08509 source file (2020-12-30)
Supplement: Supplementary file 1 [file appendix_preliminaries.tex]

% !TEX root = supplementary.tex

\section{Preliminary Claims for the Fast Rates}
\label{app:prel}

\subsection{Preliminary Lemmas}
\begin{lemma}
\label{lemma:coefs}
The diagonal coefficients of $\op\inv$ can be computed as follows:
\[\forall i \in [d], \
\op\inv_{ii}=\sum_{j=1}^d \dfrac{\sig_j \Cof(\bX_0\T)_{ij}^2}{\det(\bX_0^T\bX_0)}\dfrac{1}{p_j}.\]
\end{lemma}
\begin{proof}
We suppose that $\forall i \in [d], \ p_i \neq 0$ so that $\op$ is invertible.

We know that $\Omega(p)^{-1}=\dfrac{\mbox{Com}(\Omega(p))\T}{\det(\Omega(p))}$.

\begin{align}
\det(\op)&=\det\left(\sum_{k=1}^d \dfrac{p_k X_k X_k\T}{\sig_k}\right)\\
&=\det((\sqrt{T\inv}\bX)\T \sqrt{T\inv}\bX)\\
&=T^{-d}\det(\bX\T)^2 \\
&=T^{-d}\begin{vmatrix}
 & \vdots &  \\
\tilde{X}_1 & \vdots & \tilde{X}_d\\
 & \vdots & \
\end{vmatrix}^2 \\
&=\begin{vmatrix}
 & \vdots &  \\
\dfrac{\sqrt{p_1}}{\sigma_1} X_1 & \vdots & \dfrac{\sqrt{p_d}}{\sigma_d} X_d\\
 & \vdots & \
\end{vmatrix}^2\\
&=\det(\bX_0)^2 \dfrac{p_1}{\sig_1} \cdots \dfrac{p_d}{\sig_d}.
\end{align}

We now compute $\Com(\op)_{ii}$. We have $\Com(\op)=\Com(T^{-1/2}\bX\T T^{-1/2}\bX)=\Com(T^{-1/2}\bX\T)\Com(T^{-1/2}\bX\T)\T$.

Let us note $M \doteq T^{-1/2}\bX =\begin{pmatrix}
\cdots & \dfrac{\sqrt{p_1}}{\sigma_1}X_1\T & \cdots \\
& \vdots & \\
\cdots & \dfrac{\sqrt{p_K}}{\sigma_K}X_1\T & \cdots
\end{pmatrix}$.

Therefore
\begin{align}
\Com(\op)_{ii}&=\sum_{j=1}^d \Com(M\T)_{ij}^2\\
&=\sum_{j=1}^d \prod_{k \neq j}\dfrac{p_k}{\sig_k} \Cof(\bX_0\T)_{ij}^2.
\end{align}

Finally,
\[
\op\inv_{ii}=\sum_{j=1}^d \dfrac{\sig_j \Cof(\bX_0\T)_{ij}^2}{\det(\bX_0\T\bX_0)}\dfrac{1}{p_j}.
\]
\end{proof}

The following lemma is a restatement of Lemma~\ref{lemma:L}.
\begin{lemma}
\label{lemma:L_supp}
We have, for all $p \in \Delta^d$,
\[
L(p)=\dfrac{1}{\det(\bX_0\T\bX_0)}\skd \dfrac{\sig_k}{p_k} \Cof(\bX_0\bX_0\T)_{kk}.
\]
\end{lemma}

\begin{proof}
Using Lemma~\ref{lemma:coefs} we obtain
\begin{align}
L(p)&=\Tr(\op\inv)\\&=\sum_{k=1}^d \op\inv_{kk} =\dfrac{1}{\det(\bX\T\bX)}\skd \dfrac{\sig_k}{p_k} \sum_{i=1}^d \Cof(\bX_0\T)_{ik}^2 =\dfrac{1}{\det(\bX_0\T\bX_0)}\skd \dfrac{\sig_k}{p_k} \Com(\bX_0\bX_0\T)_{kk}.
\end{align}
\end{proof}

\begin{lemma}
\label{lemma:pstar}
For all $k \in [d]$, we have
\[
p\st_k=\dfrac{\sigma_k \sqrt{\Cof(\Gamma)_{kk}}}{\sum_{i=1}^d \sigma_i \sqrt{\Cof(\Gamma)_{ii}}},
\]
where $\Gamma=\Gram(X_1,\dots,X_d)$.
\end{lemma}

\begin{proof}
We want to minimize $L$ over the simplex.
Using KKT conditions, we obtain that all $\dfrac{\partial L(p)}{\partial p_k}$ have to be equal. Therefore there exists $\lambda$ such that for all $k \in [K]$, $\dfrac{\Cof(\Gamma)_{kk} \sig_k}{\det(\Gamma)p_k^2}=\lambda$ and finally
\[
p\st_k=\dfrac{\sigma_k \sqrt{\Cof(\Gamma)_{kk}}}{\sum_{i=1}^d \sigma_i \sqrt{\Cof(\Gamma)_{ii}}}>0.
\]
\end{proof}

\begin{lemma}
\label{lemma:strong}
$L$ is strongly convex on $\Dd$, with strong convexity parameter \[\mu=\dfrac{2}{\det(\Gamma)}\min_i \Com(\Gamma)_{ii}\sig_i.\]
\end{lemma}

\begin{proof}
We have, using Lemma~\ref{lemma:L}, that $\nabla^2 L(p)$ is a diagonal matrix and that for all $i\in[d]$, \[\nabla^2_{ii} L(p)=\dfrac{\Com(\Gamma)_{ii}\sig_i}{\det(\Gamma)}\dfrac{2}{p_i^3}\geq \dfrac{2\ \Com(\Gamma)_{ii}\sig_i}{\det(\Gamma)}.\]
\end{proof}

\begin{lemma}
\label{lemma:eta}
Let $\eta \doteq \dist(p\st,\partial \Dd)$ be the distance from $p\st$ to the boundary of the simplex.
We have
\[
\eta=\sqrt{\dfrac{K}{K-1}}\dfrac{\min_i \sigma_i \sqrt{\Cof(\Gamma)_{ii}}}{\sum_{k=1}^d \sigma_k \sqrt{\Cof(\Gamma)_{kk}}}.
\]
\end{lemma}
\begin{proof}
This is immediate with Lemma~\ref{lemma:pstar} since $\eta = \sqrt{\dfrac{K}{K-1}}\min_i p_i\st$.
\end{proof}

\subsection{Proof of Lemma~\ref{lemma:smooth_bandit}}

\begin{proof}
We use the fact that for all $i \in [d]$, $p_i \geq p^o_i/2$.
As in the proof of Lemma~\ref{lemma:strong} we have that for all $i\in[d]$, \[\nabla^2_{ii} L(p)=\dfrac{\Cof(\Gamma)_{ii}\sig_i}{\det(\Gamma)}\dfrac{2}{p_i^3}\leq \dfrac{2\ \Cof(\Gamma)_{ii}\sig_i}{\det(\Gamma) (p^o_i/2)^3}.\]
We have $p^o_k=\dfrac{\osig_k \sqrt{\Cof(\Gamma)_{kk}}}{\sum_{i=1}^d \osig_i \sqrt{\Cof(\Gamma)_{ii}}}$ which gives
\[
\nabla^2_{ii} L(p) \leq 16 \dfrac{\sigma_{\max}^2 \left(\sum_{k=1}^d \osig_k \sqrt{\Cof(\Gamma)_{kk}}\right)^3}{\det(\Gamma)\osig_{\min}^3\sqrt{\min_k \Cof(\Gamma)_{kk}}}\doteq C_S.
\]
And consequently $L$ is $C_S$-Lipschitz smooth.

We can obtain an upper bound on $C_S$ using Corollary~\ref{cor:var_conc}, which tells that $\sigma_k/2\leq \osig_k \leq 3\sigma_k/2$:
\[
C_S \leq 432 \dfrac{\sigma_{\max}^2 \left(\sum_{k=1}^d \sigma_k \sqrt{\Cof(\Gamma)_{kk}}\right)^3}{\det(\Gamma)\sigma_{\min}^3\sqrt{\min_k \Cof(\Gamma)_{kk}}}.
\]
\end{proof}
